# Supplementary material for: QMDB: Quick Merkle Database
Source: arXiv:2501.05262 source file (2025-02-01)
Supplement: Supplementary file 1 [file appendix.tex]

Appendix
[TODO: Still working on appendices]
Indexer implementation details
Truncated hashes & Sharding. The in-memory Indexer has 65536 shards. Use hash[0..2] to pick a shard. Each shard uses hash[2..9] as a 56-bit key, and returns one or multiple 48-bit offsets in the file.
The hybrid indexer also has 65536 shards. Use hash[0..2] to pick a shard. Each shard uses hash[2..10] as 64-bit key, and returns one or multiple 48-bit offsets in the file.
Sentry nodes. Cross-shard iteration is prevented with sentry nodes. A truncated hash is used (56-bit instead of 64-bit), so the index maps 56-bit hashes to 56-bit keys. 
File setup and numbers.
For a 4TB SSD, we use 64 IFOFs, each shared by 1024 shards. The database has 65535 shards in total.

Periodic compaction. The B-tree is compacted periodically (after changes amounting to 5% of the tree’s size at the previous compaction) to eliminate memory ‘bubbles’ from deleted items and ensure continued performance. TODO: Verify or remove

Hybrid indexer implementation details
Architecture. In addition to the three components (Immutable Flash Offland Files, Overlay, Cache) mentioned, there is a fourth: ActiveBits (in DRAM). This allows the indexer to support efficient answers to key existence queries, which is a feature required by the compactor and updater (see Section X on pipelining).

Cache design. The cache stores derived results instead of the raw index data, such as:
QMDB cannot find a file offset for a 8-byte key prefix (used in reads & writes)
QMDB can find a unique file offset for a 8-byte key prefix (used in reads & writes)
QMDB finds that the preceding key for a 8-byte key prefix Y’ is X’, and knows the full 32-byte keys of X and Y (used in reads, writes, creates and deletes)

Instead of a traditional eviction policy, the cache uses the block height as an estimate of recency. The cache is divided into sub-caches with each serving only one block at a particular height. The sub-caches are evicted when the block height is more than 2 after the highest seen height.

File Structure of Entries and Twigs
[TODO: Still working on this] [Placed in files one after another, not special structure]
Things to define / describe
EntryFile
EntryCache

Be clear about which parts of the Twigs are in DRAM and which in SSD.
